# Supplementary material for: VBR: Version Based Reclamation
Source: arXiv:2107.13843 source file (2021-07-29)
Supplement: Supplementary file 1 [file appendix_example.tex]

\appendix

\section{Styles of lists, enumerations, and descriptions}\label{sec:itemStyles}

List of different predefined enumeration styles:

\begin{itemize}
\item \verb|\begin{itemize}...\end{itemize}|
\item \dots
\item \dots
%\item \dots
\end{itemize}

\begin{enumerate}
\item \verb|\begin{enumerate}...\end{enumerate}|
\item \dots
\item \dots
%\item \dots
\end{enumerate}

\begin{alphaenumerate}
\item \verb|\begin{alphaenumerate}...\end{alphaenumerate}|
\item \dots
\item \dots
%\item \dots
\end{alphaenumerate}

\begin{romanenumerate}
\item \verb|\begin{romanenumerate}...\end{romanenumerate}|
\item \dots
\item \dots
%\item \dots
\end{romanenumerate}

\begin{bracketenumerate}
\item \verb|\begin{bracketenumerate}...\end{bracketenumerate}|
\item \dots
\item \dots
%\item \dots
\end{bracketenumerate}

\begin{description}
\item[Description 1] \verb|\begin{description} \item[Description 1]  ...\end{description}|
\item[Description 2] Fusce eu leo nisi. Cras eget orci neque, eleifend dapibus felis. Duis et leo dui. Nam vulputate, velit et laoreet porttitor, quam arcu facilisis dui, sed malesuada risus massa sit amet neque.
\item[Description 3]  \dots
%\item \dots
\end{description}

\cref{testenv-proposition} and \autoref{testenv-proposition} ...

\section{Theorem-like environments}\label{sec:theorem-environments}

List of different predefined enumeration styles:

\begin{theorem}\label{testenv-theorem}
Fusce eu leo nisi. Cras eget orci neque, eleifend dapibus felis. Duis et leo dui. Nam vulputate, velit et laoreet porttitor, quam arcu facilisis dui, sed malesuada risus massa sit amet neque.
\end{theorem}

\begin{lemma}\label{testenv-lemma}
Fusce eu leo nisi. Cras eget orci neque, eleifend dapibus felis. Duis et leo dui. Nam vulputate, velit et laoreet porttitor, quam arcu facilisis dui, sed malesuada risus massa sit amet neque.
\end{lemma}

\begin{corollary}\label{testenv-corollary}
Fusce eu leo nisi. Cras eget orci neque, eleifend dapibus felis. Duis et leo dui. Nam vulputate, velit et laoreet porttitor, quam arcu facilisis dui, sed malesuada risus massa sit amet neque.
\end{corollary}

\begin{proposition}\label{testenv-proposition}
Fusce eu leo nisi. Cras eget orci neque, eleifend dapibus felis. Duis et leo dui. Nam vulputate, velit et laoreet porttitor, quam arcu facilisis dui, sed malesuada risus massa sit amet neque.
\end{proposition}

\begin{conjecture}\label{testenv-conjecture}
Fusce eu leo nisi. Cras eget orci neque, eleifend dapibus felis. Duis et leo dui. Nam vulputate, velit et laoreet porttitor, quam arcu facilisis dui, sed malesuada risus massa sit amet neque.
\end{conjecture}

\begin{observation}\label{testenv-observation}
Fusce eu leo nisi. Cras eget orci neque, eleifend dapibus felis. Duis et leo dui. Nam vulputate, velit et laoreet porttitor, quam arcu facilisis dui, sed malesuada risus massa sit amet neque.
\end{observation}

\begin{exercise}\label{testenv-exercise}
Fusce eu leo nisi. Cras eget orci neque, eleifend dapibus felis. Duis et leo dui. Nam vulputate, velit et laoreet porttitor, quam arcu facilisis dui, sed malesuada risus massa sit amet neque.
\end{exercise}

\begin{definition}\label{testenv-definition}
Fusce eu leo nisi. Cras eget orci neque, eleifend dapibus felis. Duis et leo dui. Nam vulputate, velit et laoreet porttitor, quam arcu facilisis dui, sed malesuada risus massa sit amet neque.
\end{definition}

\begin{example}\label{testenv-example}
Fusce eu leo nisi. Cras eget orci neque, eleifend dapibus felis. Duis et leo dui. Nam vulputate, velit et laoreet porttitor, quam arcu facilisis dui, sed malesuada risus massa sit amet neque.
\end{example}

\begin{note}\label{testenv-note}
Fusce eu leo nisi. Cras eget orci neque, eleifend dapibus felis. Duis et leo dui. Nam vulputate, velit et laoreet porttitor, quam arcu facilisis dui, sed malesuada risus massa sit amet neque.
\end{note}

\begin{note*}
Fusce eu leo nisi. Cras eget orci neque, eleifend dapibus felis. Duis et leo dui. Nam vulputate, velit et laoreet porttitor, quam arcu facilisis dui, sed malesuada risus massa sit amet neque.
\end{note*}

\begin{remark}\label{testenv-remark}
Fusce eu leo nisi. Cras eget orci neque, eleifend dapibus felis. Duis et leo dui. Nam vulputate, velit et laoreet porttitor, quam arcu facilisis dui, sed malesuada risus massa sit amet neque.
\end{remark}

\begin{remark*}
Fusce eu leo nisi. Cras eget orci neque, eleifend dapibus felis. Duis et leo dui. Nam vulputate, velit et laoreet porttitor, quam arcu facilisis dui, sed malesuada risus massa sit amet neque.
\end{remark*}

\begin{claim}\label{testenv-claim}
Fusce eu leo nisi. Cras eget orci neque, eleifend dapibus felis. Duis et leo dui. Nam vulputate, velit et laoreet porttitor, quam arcu facilisis dui, sed malesuada risus massa sit amet neque.
\end{claim}

\begin{claim*}\label{testenv-claim2}
Fusce eu leo nisi. Cras eget orci neque, eleifend dapibus felis. Duis et leo dui. Nam vulputate, velit et laoreet porttitor, quam arcu facilisis dui, sed malesuada risus massa sit amet neque.
\end{claim*}

\begin{proof}
Fusce eu leo nisi. Cras eget orci neque, eleifend dapibus felis. Duis et leo dui. Nam vulputate, velit et laoreet porttitor, quam arcu facilisis dui, sed malesuada risus massa sit amet neque.
\end{proof}

\begin{claimproof}
Fusce eu leo nisi. Cras eget orci neque, eleifend dapibus felis. Duis et leo dui. Nam vulputate, velit et laoreet porttitor, quam arcu facilisis dui, sed malesuada risus massa sit amet neque.
\end{claimproof}
